# Supplementary material for: Transverse Kerker Scattering for Angstrom Localization of Nanoparticles
Source: arXiv:1804.10176 source file (2018-11-12)
Supplement: Supplementary file 1 [file Supplementary.pdf]

# Supplementary Material: Transverse Kerker Scattering for Ångström Localization of Nanoparticles

Ankan Bag,[1,2] Martin Neugebauer,[1,2] Paweł Woźniak,[1,2] Gerd Leuchs,[1,2] and Peter Banzer[1,2]

[1]*Max Planck Institute for the Science of Light, Staudtstr. 2, D-91058 Erlangen, Germany*
[2]*Institute of Optics, Information and Photonics, Department of Physics, Friedrich-Alexander-University Erlangen-Nuremberg, Staudtstr. 7/B2, D-91058 Erlangen, Germany*

(Dated: October 2, 2018)

## CALCULATION OF DIRECTIVITY PARAMETERS

In order to calculate the directivity parameters $D_x$ and $D_y$ from the expansion coefficients of the scattered light defined in the manuscript, $a_{mn}^{\mathrm{sca}'}$ and $b_{mn}^{\mathrm{sca}'}$, we write the vector spherical wave functions of the third kind in a plane wave representation [1]:

$$\begin{aligned}\mathbf{M}_{mn}^{i}(\mathbf{r}) &= \frac{(-\imath)^{n}\gamma_{mn}}{2\pi}\int_{\Omega_k} e^{\imath\mathbf{kr}}\mathbf{X}_{mn}^{2}(\theta_k,\phi_k)\,d\Omega_k,\\ \mathbf{N}_{mn}^{i}(\mathbf{r}) &= \frac{(-\imath)^{n-1}\gamma_{mn}}{2\pi}\int_{\Omega_k} e^{\imath\mathbf{kr}}\mathbf{X}_{mn}^{1}(\theta_k,\phi_k)\,d\Omega_k.\end{aligned} \tag{S1}$$

the indices $m$ and $n$ denote the multipole order, $\mathbf{X}_{mn}^{1}(\theta,\phi)$ and $\mathbf{X}_{mn}^{2}(\theta,\phi)$ are vector spherical harmonics (VSH), $\gamma_{mn}$ are prefectors, and $\mathbf{k}$ represents the $k$-vector. The angular integration region $\Omega$ contains propagating and evanescent waves with $\phi \in [0, 2\pi]$ and $\theta \in [0, \pi/2 - \imath\infty]$ for $z > 0$ and $\theta \in [\pi/2 - \imath\infty, \pi]$ for $z < 0$.

In the manuscript, we define the directivity parameters as normalized difference between the light scattered into opposite directions. Thereby, we consider the scattered light after transmission through the interface at the critical angle. The light that is transmitted into this angular regime corresponds to the light propagating parallel to the interface before transmission. Within the angular spectrum representation, this corresponds to $\theta = \pi/2$. Without loss of generality, we calculate the the intensity values $I_1$, $I_2$, $I_3$ and $I_4$ with respect to the $x$- ($\phi_1 = 0$ and $\phi_3 = \pi$) and $y$-directions ($\phi_2 = 3\pi/2$ and $\phi_4 = \pi/2$). The auxiliary scattered field $\mathbf{E}^{\mathrm{sca}'}$ before transmission is defined by Eq. (2) of the manuscript. In the far-field approximation [1], the electric field distribution reads

$$\mathbf{E}_{\mathrm{far}}^{\mathrm{sca}'}(\pi/2,\phi_j) \approx \sum_{n=1}^{\infty}\sum_{m=-n}^{n}\gamma_{mn}\left[\imath^{-n-1}b_{mn}^{\mathrm{sca}'}\mathbf{X}_{mn}^{2}(\pi/2,\phi_j) + \imath^{-n}a_{mn}^{\mathrm{sca}'}\mathbf{X}_{mn}^{1}(\pi/2,\phi_j)\right]. \tag{S2}$$

Since the transmission through the interface introduces polarization dependent Fresnel transmission coefficients [2], we need to perform the corresponding polarization projections to determine the intensity values $I_1$, $I_2$, $I_3$ and $I_4$ [3]:

$$\begin{aligned}I_1 &\propto \left|t_p\hat{\mathbf{e}}_p\mathbf{E}_{\mathrm{far}}^{\mathrm{sca}'}(\pi/2,0)\right|^2 + \left|t_s\hat{\mathbf{e}}_s\mathbf{E}_{\mathrm{far}}^{\mathrm{sca}'}(\pi/2,0)\right|^2,\\ I_2 &\propto \left|t_p\hat{\mathbf{e}}_p\mathbf{E}_{\mathrm{far}}^{\mathrm{sca}'}(\pi/2,3\pi/2)\right|^2 + \left|t_s\hat{\mathbf{e}}_s\mathbf{E}_{\mathrm{far}}^{\mathrm{sca}'}(\pi/2,3\pi/2)\right|^2,\\ I_3 &\propto \left|t_p\hat{\mathbf{e}}_p\mathbf{E}_{\mathrm{far}}^{\mathrm{sca}'}(\pi/2,\pi)\right|^2 + \left|t_s\hat{\mathbf{e}}_s\mathbf{E}_{\mathrm{far}}^{\mathrm{sca}'}(\pi/2,\pi)\right|^2,\\ I_4 &\propto \left|t_p\hat{\mathbf{e}}_p\mathbf{E}_{\mathrm{far}}^{\mathrm{sca}'}(\pi/2,\pi/2)\right|^2 + \left|t_s\hat{\mathbf{e}}_s\mathbf{E}_{\mathrm{far}}^{\mathrm{sca}'}(\pi/2,\pi/2)\right|^2.\end{aligned} \tag{S3}$$

Finally, we calculate the theoretical directivity parameters defined for the $x$- and $y$-directions,

$$\begin{aligned}D_x = \frac{I_3 - I_1}{I_{\mathrm{tot}}},\ D_y = \frac{I_2 - I_4}{I_{\mathrm{tot}}}\\ \text{where } I_{\mathrm{tot}} = \frac{I_1 + I_2 + I_3 + I_4}{2}.\end{aligned} \tag{S4}$$

### Position dependent directional scattering

Since we want to investigate how strong a small shift of the particle changes the far-field directivity parameters, we need to apply the translation addition theorems [4] to the incoming field described by first order regular (Rg) vector spherical wave functions to take into account the shift of the coordinate system of the scatterer from $\mathbf{r} = (r, \theta, \phi)$ to $\mathbf{r}'' = (r'', \theta'', \phi'') = \mathbf{r} - \mathbf{a}$, with $\mathbf{a} = (r_a, \theta_a, \phi_a)$ as displacement vector. Here, we consider displacements

in the $x$-$y$-plane only, which implies that $\theta_a = \pi/2$.

Now we write the incoming field distribution of the original coordinate frame ($Rg\mathbf{M}_{mn}$ and $Rg\mathbf{N}_{mn}$) in the basis of the new coordinates frame ($Rg\mathbf{M}''_{\mu\nu}$ and $Rg\mathbf{N}''_{\mu\nu}$),

$$\mathbf{E}_{in} = \sum_{\nu=1}^{\infty} \sum_{\mu=-\nu}^{\nu} A''_{\mu\nu} Rg\mathbf{N}''_{\mu\nu} + B''_{\mu\nu} Rg\mathbf{M}''_{\mu\nu}. \tag{S5}$$

The relation between the new and the old expansion coefficients can be written in matrix form [3]:

$$\begin{pmatrix} \mathbf{A}'' \\ \mathbf{B}'' \end{pmatrix} = \begin{pmatrix} \hat{\mathbf{Tr}}^{11} & \hat{\mathbf{Tr}}^{12} \\ \hat{\mathbf{Tr}}^{21} & \hat{\mathbf{Tr}}^{22} \end{pmatrix} \begin{pmatrix} \mathbf{A} \\ \mathbf{B} \end{pmatrix}, \tag{S6}$$

with $\hat{\mathbf{Tr}}^{11} = \hat{\mathbf{Tr}}^{22} \equiv \hat{\mathbf{Tr}}^{\alpha}$ and $\hat{\mathbf{Tr}}^{12} = \hat{\mathbf{Tr}}^{21} \equiv \hat{\mathbf{Tr}}^{\beta}$ as submatrices of the full translation matrix $\hat{\mathbf{Tr}}$. The elements of the sub matrices are given by [3, 4]

$$\begin{aligned} \alpha_{\mu\nu}^{mn} &= \sum_p a_{mn}^{\mu\nu}(p)\, j_p(k\Delta\rho)\, P_p^{m-\mu}(0)\, e^{\imath(m-mu)\phi_a}, \\ \beta_{\mu\nu}^{mn} &= \sum_p b_{mn}^{\mu\nu}(p)\, j_p(k\Delta\rho)\, P_p^{m-\mu}(0)\, e^{\imath(m-mu)\phi_a}, \end{aligned} \tag{S7}$$

where $a_{mn}^{\mu\nu}$ and $b_{mn}^{\mu\nu}$ are transition matrix elements [4], $j_i$ represents spherical Bessel-functions, and $P_i^j(x)$ denotes the associated Legendre polynomials. The range of the index $p$ is defined by $|\nu - n| \leq p \leq \nu + n$. Now, we can calculate the scattered light for shifted particle positions similar to Eq. (2) of the manuscript [3]:

$$\mathbf{E}^{\text{sca}''} = \hat{\mathbf{T}}_{\text{eff}} \hat{\mathbf{Tr}} \mathbf{E}^{\text{inc}}. \tag{S8}$$

Finally, we perform a theoretical calibration of the directivity parameter similar to the experiment, where we scan the particle across the focal plane and calculate the directivity parameters for each position of the particle. The wavelength dependent sensitivity parameter $S_{x(y)}$ or the average change in $D_x$ and $D_y$ (as defined in Eqs. (S4)) per nanometer displacement—$|S_{x(y)}|$ is plotted in Fig. 3(h) of the manuscript.

## METHODS

### A. Experimental set-up

A linearly polarized fundamental Gaussian beam for the wavelength range from $510-660$ nm is converted into a radially or azimuthally polarized beam by a liquid-crystal polarization converter (q-plate) [5]. The beam is then guided into a microscope objective with an numerical aperture (NA) of 0.9 and an entrance aperture radius of 1.8 mm. The set-up is aligned for each wavelength in a way that the particle is always placed in the focal plane. The radius of the incoming beam before it is guided to the objective varies with wavelength but always fills the objective aperture. A single spherical silicon nanoparticle with diameter d=156 nm (with an extra silicon-dioxide shell of estimated thickness 6 nm) on a glass substrate is scanned through the focal plane by a high-precision 3D piezo-stage, and the transmitted light is collected with an oil-immersion objective with NA=1.3 from below. The angular intensity distribution of the transmitted light is detected by imaging the backfocal plane of the oil-immersion objective onto a CCD camera. The larger collection NA of the oil-immersion objective allows us to access the supercritical angular region, where light scattered from the nanosphere is collected without interfering with the transmitted light (see Fig. S1).

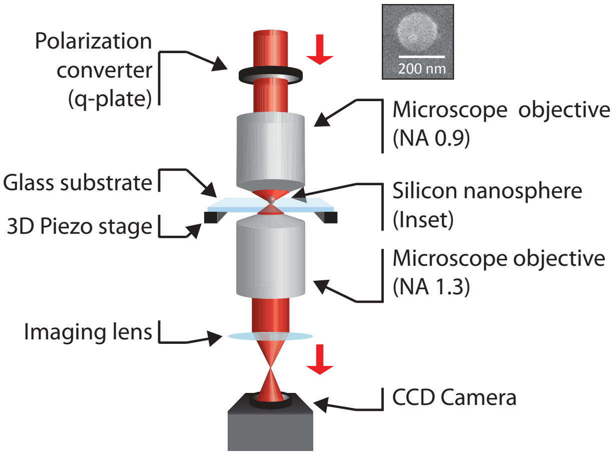


FIG. S1. Schematic of the experimental setup. Inset: SEM image of the silicon nanoparticle utilized in the experiment. Estimated size parameters: core diameter of 156 nm and a silicon-dioxide shell of 6 nm.

The tunable light source used is an NKT Photonics SuperK Extreme & SpectraK Dual with a spectral bandwidth of approximately 1 nm. The focusing objective above the nanoparticle is Leica HCX PL FLUOTAR 100 × /0.90 POL 0/D and the objective for collecting light below is Leica HCX PL FLUOTAR 100 × /1.30 OIL. The 3D piezo stage used to control the movement the nanoparticle is PI P-527. The CCD camera used to image the backfocal plane is The Imaging Source DMK 23U618.

### B. Data acquisition

For calibration, we raster scan our nanoparticle using the aforementioned 3D piezo-stage in a 100 nm × 100 nm area around the optical axis with a step size of 10 nm. The on-axis position corresponds to zero directivity and serves as our reference point. For each position, we capture backfocal plane images with 1 ms exposure time. For each position, we take into account more than 50 measurements for the calibration and the calculation

of the error bars. We find linear dependence of the directivity with the radial distance from the optical axis for a radius of at least 30 nm (for azimuthally polarized 545 nm beam). This linear dependence is beam and wavelength dependent and continues also for even longer distances. For example for a radially polarized beam at 625 nm, the directivity changes linearly at least up to a radial distance of 50 nm from the optical axis. For each wavelength, for both the radially and azimuthally polarized beam, we obtain the calibration curve and its slope $S_{x(y)}$ (directivity change per nm along $x$- and $y$-direction). The calibration curve is shown in Fig. 3(h) in the main manuscript, where we also compare the results from the numerical calculation.

Instability of our experimental set-up causes an uncertainty of $\pm 4$ nm regarding the position of the nanoparticle relative to the optical axis. For exemplary displacement measurements, we raster scan our nanosphere with a 2 nm step size within the region of $x = [-20, 20]$ nm and $y = [-20, 20]$ nm around the optical axis. Within this region, directivity changes linearly with distance for all wavelengths and for both the radially and azimuthally polarized beam. For each position within this area, we capture images with 1 ms exposure time, where the actual position information gets encoded in each of the backfocal plane images. This leads to a collection of particle positions, some of which are only few Ångström apart owing to the positioning inaccuracy of our system. We use the images recorded for particle positions, which are less than 1 nm apart from each other to showcase experimentally that by using our scheme it is possible to resolve those displacements with localization accuracies on the sub-Ångström level.

### C. Data processing

Within the backfocal plane, the four solid angles corresponding to $\Delta\tilde{I}_j$s ($j \in [1, 4]$) are defined by an azimuthal angular range of $\Delta\Phi = 45°$ each and by NA∈[0.98, 1.03] (see Fig. S2 and Fig. 4 of the main manuscript). These angular ranges are chosen because, firstly, the scattering signal from a dipole on an interface is mostly confined around an NA=1 (critical angle) [2]. The scattering signal drops rapidly with increasing angular distance from NA=1. Hence, by choosing the aforementioned angular ranges, a better signal-to-noise ratio is achieved. Secondly, we chose the angular region such that the signal is not only strong but also fairly uniform across the depicted areas in the BFP. This way, the error analysis for calculating the accuracy of this method can be significantly simplified. This allows us to calculate the mean and the standard error of the mean from the pixel intensity distributions for each of those angular regions, which we then use to calculate the relative displacement and the uncertainty or accuracy of our measurement.

For a nanoparticle position pair in the $xy$-plane, $\Delta\tilde{I}$ $(= [\tilde{I}(x_1, y_1) - \tilde{I}(x_2, y_2)]/I_{\text{tot}})$ represents the differential backfocal plane intensity distribution. For our nanoparticle movement along $\pm x$-direction, the observed Kerker scattering is along $\pm k_x$, hence, to calculate the $x$-component of the displacement, we consider the angular regions $j = 1, 3$ (denoted by dashed black border in Fig. S2). $\Delta I_1$ and $\Delta I_3$ are the expectation value of the fitted Gaussian to the pixel-wise intensity distribution of $\Delta\tilde{I}_1$ and $\Delta\tilde{I}_3$ respectively. Similarly, for $j = 2, 4$ (denoted by solid black border), we obtain $\Delta I_2$ and $\Delta I_4$ to calculate the $y$-component of the displacement. They follows as

$$\Delta x = \frac{\Delta I_3 - \Delta I_1}{S_x}, \Delta y = \frac{\Delta I_2 - \Delta I_4}{S_y}. \tag{S9}$$

where $S_x$ and $S_y$ are the sensitivity (slopes of the directivity curves per nm displacement) along $x$- and $y$-direction. To estimate the error in calculating $\Delta x$, we use the standard error propagation formula for a functional dependence of the type $f = \frac{A}{B}$. In the considered case,

$$\begin{aligned} A &= \Delta I_3 - \Delta I_1, \\ B &= S_x. \end{aligned} \tag{S10}$$

We calculate the standard error of the mean $\sigma_{M,j} = \sigma_j / \sqrt{\#\text{ of pixels}_j}$ for the $j$th region to estimate the error

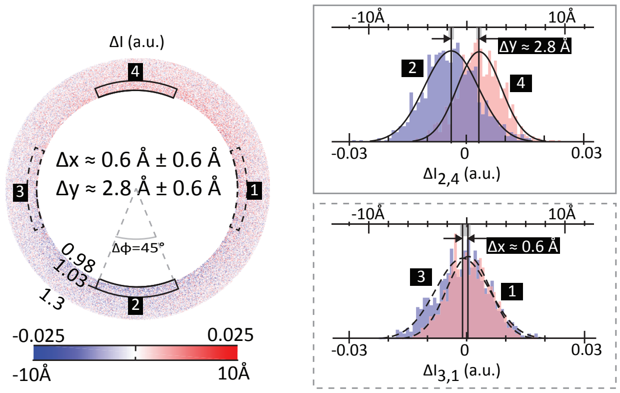


FIG. S2. (left) Differential backfocal plane intensity ($\Delta\tilde{I}$) distribution for NA∈[0.98, 1.3]. The four intensity distributions $\Delta\tilde{I}_j, j \in [1, 4]$ considered for calculating displacements, $\Delta x$ and $\Delta y$, corresponds to the four bordered region given by $\Delta\phi = 45°$ and NA∈[0.98, 1.03] along $\pm k_x$ (dashed border) and $\pm k_y$ (solid border). Number of pixel in each region $j, j \in [1, 4]$ is in the order of $10^3$. (right-top) Histogram plots and Gaussian fits of $\Delta\tilde{I}_2$ and $\Delta\tilde{I}_4$ and the peak-to-peak distance between two Gaussian fits gives us relative displacement along $y$-direction, $\Delta y = 2.8$ Å. (right-bottom) Similarly, $\Delta x = 0.6$ Å is obtained from the histogram plots and Gaussian fits of $\Delta\tilde{I}_1$ and $\Delta\tilde{I}_3$.

in $\Delta I_j$, $j = 1, 3$. Hence,

$$\begin{aligned} &\text{error in A} = \Delta I_3 - \Delta I_1 \text{ is } \sqrt{[\sigma_{M,3}^2 + \sigma_{M,1}^2]} \\ &\text{error in B} = S_x \text{ is } \Delta S_x, \end{aligned} \tag{S11}$$

where $\Delta S_x$ is obtained from the fitting error of the slope represented as error bars in Fig. 3(h) in the main manuscript. Hence, error in calculating $\Delta x$ follows as

$$\begin{aligned} &\frac{\text{A}}{\text{B}} \sqrt{\left[\frac{\text{error in A}}{\text{A}}\right]^2 + \left[\frac{\text{error in B}}{\text{B}}\right]^2} \\ &= \frac{\Delta I_3 - \Delta I_1}{S_x} \sqrt{\left[\frac{\sqrt{\sigma_{M,3}^2 + \sigma_{M,1}^2}}{\Delta I_3 - \Delta I_1}\right]^2 + \left[\frac{\Delta S_x}{S_x}\right]^2} \\ &= \sqrt{\left[\frac{\sqrt{\sigma_{M,3}^2 + \sigma_{M,1}^2}}{S_x}\right]^2 + \left[\frac{\Delta S_x.(\Delta I_3 - \Delta I_1)}{{S_x}^2}\right]^2}. \end{aligned} \tag{S12}$$

Similarly, following Eqn. S12, we estimate the error in calculating $\Delta y$. It is worth mentioning that, while the camera noise contribution ($\sigma_{M,j}$) are fixed for this experiment and can be improved significantly by using a better camera, the error $\Delta S_x$ becomes less and less with more number of measurement used for calibration. In our experiment, we considered more than 50 measurement values for each data point in the calibration curves (two of those are shown in the inset of Fig. 3(h) in the main manuscript). In Fig. S2, we reconsider the right-most example of Fig. 4 of the main manuscript and in detail show the histogram plots and Gaussian fits of $\Delta \tilde{I}_j$s, $j \in [1, 4]$, of the differential backfocal plane image. Following Eqn. [9-12], we calculate the relative displacements $\Delta x = 0.6\,\text{Å}$, $\Delta y = 2.8\,\text{Å}$ with an uncertainty of $0.6\,\text{Å}$.


[1] L. Tsang, J. A. Kong, and K.-H. Ding, *Scattering of Electromagnetic waves*, 1st ed. (John Wiley and Sons, Inc., New York, 2000).

[2] L. Novotny and B. Hecht, *Principles of Nano-Optics*, 2nd ed. (Cambridge University Press, Cambridge, 2006).

[3] T. Bauer, S. Orlov, U. Peschel, P. Banzer, and G. Leuchs, Nature Photon. **8**, 23 (2014).

[4] O. Cruzan, Quart. Appl. Mates. **20**, 33 (1961).

[5] L. Marrucci, C. Manzo, and D. Paparo, Phys. Rev. Lett. **96**, 163905 (2006).
